# Supplementary material for: ACE: Adversarial Correspondence Embedding for Cross Morphology Motion Retargeting from Human to Nonhuman Characters
Source: arXiv:2305.14792 source file (2023-05-24)
Supplement: Supplementary file 1 [file appendix.tex]

\newpage
\appendix

\section{Appendix}

\subsection{Sampling for pretraining motion prior}
\ref{}
\begin{algorithm}[t]

\label{algo:sampling}

\caption{Collect data for pretraining controllers} 
\label{Algo:SamplingAlgo}
\begin{algorithmic}

\While {Dataset $\Omega_L$ not \textbf{FULL}} \Comment{Collect Loco Data}
\State {$x_0  \gets$  Initialize robot}
\State {$t \gets 0$ }
\State {$\pi^{L,exp}  \gets$  Initialize designed kinematics controller}
    \While{Episode not \textbf{END}}
        \If {t \% 20 ==0}
            \State {$z^L_{t+1} \gets$ randomly sample commands}
        \EndIf
        \State {$x_{t+1} \gets \pi^{L,exp}(z^L_{t+1}, x_{t})$ }
        \State {$t \gets t +1$ }
        \State {$\Omega_L \gets \Omega_L \cup \{ (x_{t+1}, z^L_{t+1}, x_{t}   )\}$ }
    \EndWhile
\EndWhile

\\
\While {Dataset $\Omega_M$ not \textbf{FULL}} \Comment{Collect Mani Data}

 \State {$x_0  \gets$  Sample robot arm initial pose until no self-collision}
 \State {$t \gets 0$ }
 \State {$\pi^{M,exp}  \gets$  Max pose clip check function}
 \State {self-collision $\gets$ \textbf{FALSE}}

 \While{self-collision is \textbf{FALSE}}

\State {$\mathbf{z^M_{t+1}}  \gets$  Sample desired pose until no self-collision}
\State {$x_{t+1} \gets \pi^{M,exp}(z^M_{t+1}, x_{t})$ }
\State {$t \gets t +1$ }
\State {$\Omega_M \gets \Omega_M \cup \{ (x_{t+1}, z^M_{t+1}, x_{t}   )\}$ }
 \State {self-collision $\gets$ check self-collision}
 \EndWhile
\EndWhile

\end{algorithmic}
\end{algorithm}
